# Supplementary material for: Intraoperative robotic-assisted large-area high-speed microscopic imaging and intervention
Source: arXiv:1808.04146 ancillary file (2018-08-13)
Supplement: Supplementary file 1 [file SupplementaryMaterials.pdf]

# Intraoperative robotic-assisted large-area high-speed microscopic imaging and intervention - Supplementary material

**Petros Giataganas, Michael Hughes, Christopher J. Payne, Piyamate Wisanuvej, Burak Temelkuran, and Guang-Zhong Yang**

## 1 Mechanical Design of the Robotic Scanning Device

An exploded view of the robotic scanning device is presented in Fig. S1. The cantilevered tube shaft is mounted rigidly in the back-end of the tubular chassis. Two micro-motors are fixed on the motor base, on the front-end of the tubular chassis, to drive the two cam rollers. A V-profiled steel cam is welded to the tube shaft; it is engaged by the two steel cam rollers with tip mounted bearings that exert lateral forces onto the cantilevered tube. A probe mounting tip, separating the optical fibre and the ablation fibre, is attached to the distal end of the tube shaft.

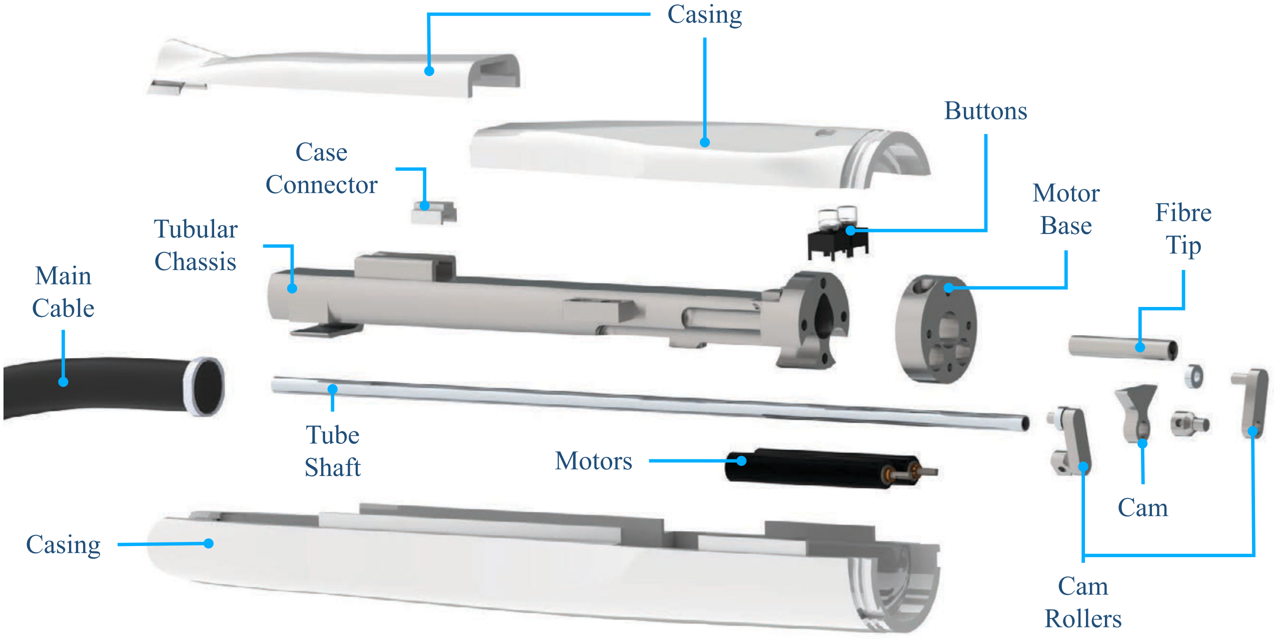


**Figure S1.** Exploded view of the handheld robotic scanning device.

## 2 Kinematic model analysis

For the kinematic analysis of the device, a two-step approach is used. Initially, using a geometric method, presented in Fig. S2, the two motor angles $\theta_1$ and $\theta_2$ are used to find the position $P(x,y)$ of the shaft centre with respect to the coordinate system at the origin point $O$. Then, we can calculate the tip end-effector position using a simple tube deflection method. The derivation of the geometric solution proceeds as follows:

- We assume that the angle $\theta_1$ is calculated as the angle $\angle DAC$ where AD is the perpendicular line from A to the line connecting the two motor centres. Similarly, we assume that the angle $\theta_2$ is calculated as the angle $\angle KNL$ where NK is the perpendicular line from N to the line connecting the two motor centres.
- The origin of the kinematic model is considered the origin point $O$, which is the middle point of the line connecting the two motors. The result of the first part of the kinematic model analysis is the coordinates $x, y$ of the point P, which is the centre of the device's shaft.

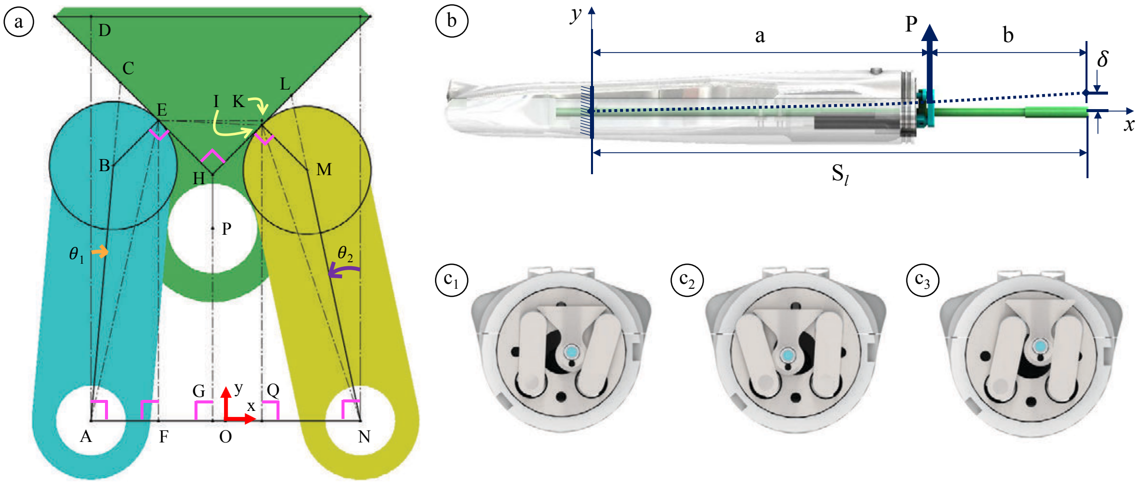


**Figure S2.** (a) Geometric model for kinematic analysis of the two roller - cam system. The geometric solution finds the relation between the two motor angles $\theta_1$ and $\theta_2$ and the position $P(x,y)$ of the shaft centre in relation to the coordinate system at the origin point O. (b) Side view of the instrument presenting the tube deflection at the tip of the device, its fixing point and the load position P. (c) Three different scanning positions presenting the steel level positions with the resulting tip position.

From the design characteristics we know the following: lever length $AB = MN = l$, bearing radius $BE = MI = r$, motor centre distance $AN = m$, distance $HP = Di$, $\angle CHL = \pi/2$ and $\angle BEH = \pi/2$, $\angle HIM = \pi/2$ since $E$ and $I$ are the contact points between the bearings on the rollers and the cam.

The polygon's ABEHG angles have sum $3\pi$. Therefore:

$$\angle ABE = 3\pi - \angle BEH - \angle EHG - \angle HGA - \angle GAB = 3\pi - \pi/2 - 3\pi/4 - \pi/2 - (\pi/2 - \theta_1) = 3\pi/4 + \theta_1 \tag{2.1}$$

Similarly for the polygon MIHGN:

$$\angle IMN = 3\pi/4 + \theta_2 \tag{2.2}$$

From (2.1), we have $\angle CBE = \pi - \angle ABE = \pi/4 - \theta_1$, and from (2.2), we have $\angle IML = \pi - \angle IMN = \pi/4 - \theta_2$. Using simple trigonometric equations, we proceed as follows:

$$BC = BE/cos(\angle CBE) = r/cos(\pi/4 - \theta_1) \tag{2.3}$$

$$ML = MI/cos(\angle IML) = r/cos(\pi/4 - \theta_2) \tag{2.4}$$

$$CE = \sqrt{BC^2 - BE^2} = \sqrt{BC^2 - r^2} \tag{2.5}$$

$$IL = \sqrt{ML^2 - MI^2} = \sqrt{ML^2 - r^2} \tag{2.6}$$

$$AE = \sqrt{(AB^2 + BE^2) - 2(AB)(BE)cos(\angle ABE)} = \sqrt{(l^2 + r^2) - 2lrcos(\angle ABE)} \tag{2.7}$$

$$NI = \sqrt{(NM^2 + NI^2) - 2(NM)(MI)cos(\angle IMN)} = \sqrt{(l^2 + r^2) - 2lrcos(\angle IMN)} \tag{2.8}$$

$$\angle BAE = \arcsin((BE/AE)\sin(\angle ABE)) \tag{2.9}$$

$$\angle INM = \arcsin((MI/NI)\sin(\angle NMI)) \tag{2.10}$$

$$\angle EAF = \pi - (\theta_1 + \angle BAE) \tag{2.11}$$

$$\angle INQ = \pi - (\theta_2 + \angle INM) \tag{2.12}$$

$$EK = FQ = AN - AF - NQ = AN - (AE/cos(\angle EAF)) - (NI/cos(\angle INQ)) \tag{2.13}$$

$$KI = FE - QI = (AE/sin(\angle EAF)) - (NI/sin(\angle INQ)) \tag{2.14}$$

$$EI = \sqrt{EK^2 + KI^2} = \sqrt{FQ^2 + KI^2} \tag{2.15}$$

$$\angle KEI = \arccos(EK/EI) \tag{2.16}$$

$$\angle IEH = \pi/2 - (\angle EHI/2) - \angle KEI \tag{2.17}$$

$$EH = EIcos(\angle IEH) \tag{2.18}$$

$$IH = EIsin(\angle IEH) \tag{2.19}$$

$$OG = -(AN/2) + AF + EHcos(\angle HEF) \tag{2.20}$$

$$GP = EF - EHsin(\angle HEF) - HP \tag{2.21}$$

Equations (2.20) and (2.21) provide the coordinates $P(x,y)$ of the shaft's centre with respect to the coordinate system at the origin point $O$.

As presented in the main manuscript, at the second step of the kinematic analysis, the tube deflection is considered to find the end-effector position at the tip of the shaft. Initially, the Cartesian coordinates $P(x,y)$ are converted to polar coordinates $P(r_p, \theta_p)$ and we compute the end deflection based on knowing the deflection part way along the tube $\delta$, using beam theory. We then convert back to Cartesian coordinates to get $P_t(x_t, y_t)$ positions at the tip. In this approach, we assume that there are no large deflections, the plane sections remain plane and the material has linear elastic behaviour. We also assume minimal z motion both at the cam deflection point and at the end deflection point. We believe that these assumptions are well within the manufacturing/assembly tolerance and hence are reasonable.

As presented in Fig. S2(b), using the beam deflection formula for concentrated load P at any point, the maximum deflection $\delta$ is calculated as:

$$\delta = \frac{Pa^2}{6EI}(3S_l - a) \tag{2.22}$$

where $S_l$ is the length of the shaft, $E = 209\,GPa$ is the elastic modulus of steel, and $I$ is the second moment of area:

$$I = \frac{\pi}{64}(OD^4 - ID^4) \tag{2.23}$$

where $OD = 3.3mm$ is the outer diameter of the tube and ID is the inner, $ID = 2.7mm$, and

$$P = \frac{6EIr_p}{2a^3} \tag{2.24}$$

Finally, the tip position $P_t(x_t, y_t)$ in Cartesian coordinates is:

$$x_t = \delta * sin(\theta_p) \tag{2.25}$$

$$y_t = \delta * cos(\theta_p) \tag{2.26}$$

By driving the instrument in a straight line within the linear workspace, the scaling factor between analog voltage inputs and the Cartesian correspondences can be calculated using the mosaic image generated. This was found to be 664 $\mu m\,V^{-1}$ for both directions. The correspondence between the motor rotations (in degrees) and the analog input voltages can be found from the following motor settings: (a) voltage range = $20V$, (b) motor increments range (without gear transmission) = 100000, (c) motor increments range (without gear transmission) per revolution = 3000 and (d) gear ratio = 256. Hence, the value of R (in degrees per volt) can be determined to be:

$$R = 360\frac{1}{256}\frac{1}{3000}\frac{100000}{20} = 2.3438^o/V \tag{2.27}$$

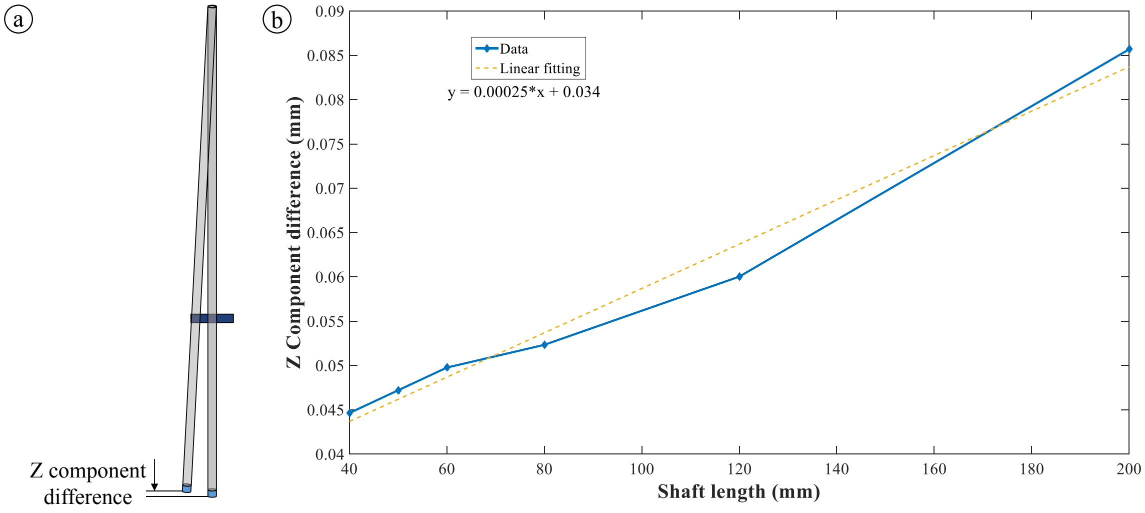


**Figure S3.** Shaft length analysis: (a) Visualisation demonstrating the change in axial position at the extremes of the instrument's workspace and (b) graph presenting the axial change versus various shaft lengths.

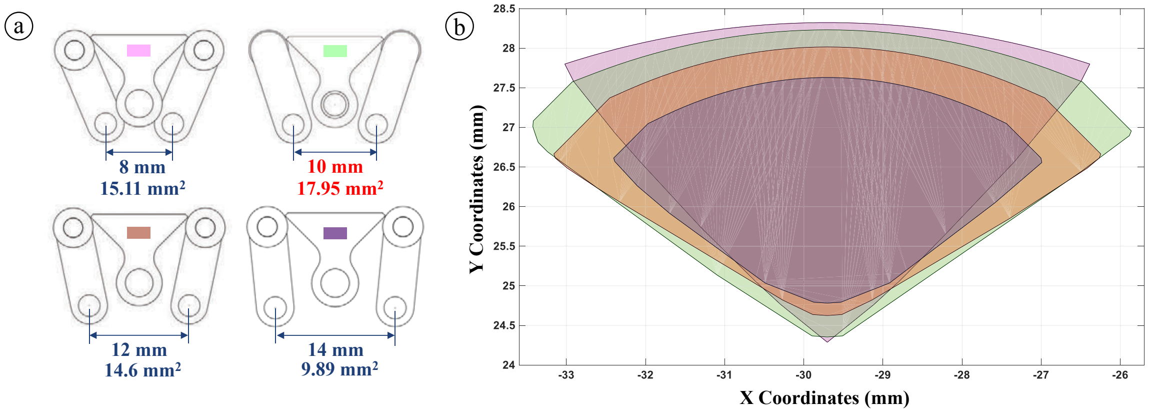


**Figure S4.** Analysis of the cam-roller mechanism positions: (a) four different position configurations explored during the analysis and (b) simulated workspace results for the four different configurations. In Fig. (b), each colour area corresponds to different configurations as presented in Fig. (a)

## 3 Mechanical Performance Evaluation and Characterisation

A CAD simulation was performed (see Fig. S3) to explore the effect of the cantilevered tube design on imaging performance. It is important that the motion of the tube tip is near planar, to avoid loss of contact between the probe and the tissue during scanning. Fig. S3(b) demonstrates that the axial difference is less than 50 $\mu m$ at the extremes of the workspace for a tube of length 58 $mm$. Simulations were also performed to ensure that the position of the motors and consequently the configuration of the cam-roller mechanism was optimised to achieve the largest possible workspace in the smallest possible overall dimensions for the actuation system. CAD simulations of four different configurations are shown in Fig. S4; a 10 $mm$ distance between the cam-roller mechanisms was chosen as it provides the largest simulated workspace (17.95 $mm^2$ - green).

## 4 Custom Tracking Rig

Mechanical performance evaluation was performed using a custom tracking system that could measure the position of the tip of the instrument with an accuracy of 7.5 $\mu m$ without imposing any additional weight on the instrument (as opposed to commercial off-the-shelf tracking systems, such as electromagnetic and optical trackers, that provide typically 100 $\mu m$ accuracy, almost half the image probe field-of-view). In the tracking system, the probe is imaged onto a monochrome, $1280 \times 1280$ $pixel$ CCD camera by an achromatic doublet lens, with all three components fixed and aligned along the axis of the scanning mechanism of the instrument, as shown in Fig. S5(a). Light was coupled into the endomicroscopy probe, making it visible on the camera.

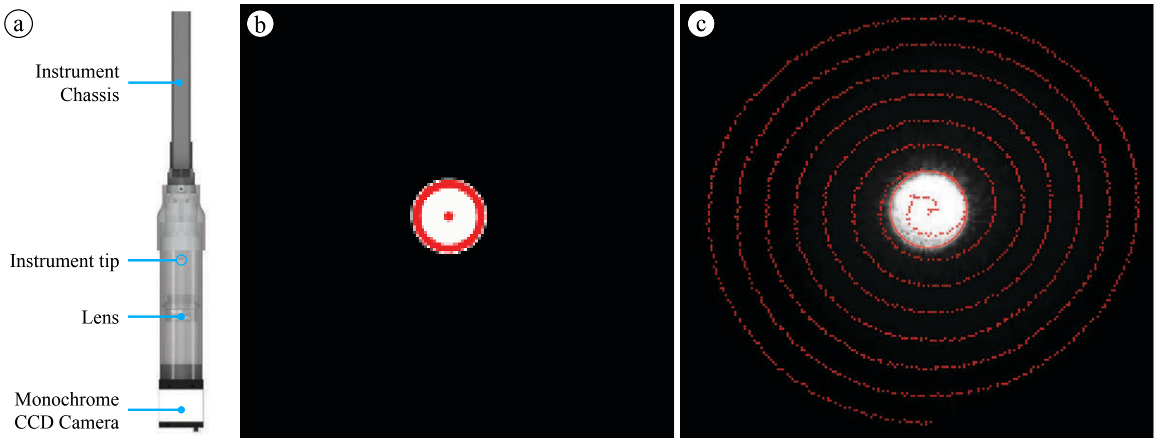


**Figure S5.** Tracking rig used for workspace and mechanical performance analysis: (a) Custom tracking rig, (b) zoomed region of the tracked tip after binary conversion showing the tracked circle and its centre, (c) zoomed image showing an example tracked spiral trajectory overlaid onto a single image of the probe tip.

The recorded image sequence showed a bright circle corresponding to the instrument's tip against a dark background, as can be seen in Fig. S5(b-c). To determine the probe tip position during scanning, each recorded frame was first converted into a binary image where the instrument's tip appears as a circle of 15 *pixels* diameter (see Fig. S5(b)). The circle was then localised using a two-stage Hough Transform method[1] (see Fig. S5(c)). Spatial calibration was performed via the known diameter of the circle, which corresponds to the fibre bundle diameter as projected onto the image plane of the endomicroscope via the distal micro-objective.

The previous circle tracking method was used to evaluate the repeatability and accuracy of the instrument. Two different scanning approaches (spiral and raster) have been evaluated. In Fig. S6 the different trajectory patterns are demonstrated; three repeats of spiral trajectories and four repeats of raster trajectories, using the same parameters across the repeats, are performed in sequence. The position errors relative to the original planned trajectory are also presented, with the maximum position error not exceeding 30 $\mu m$ and the median error across all the trajectories being 10.7 $\mu m$ with interquartile range of 7.5 $\mu m$.

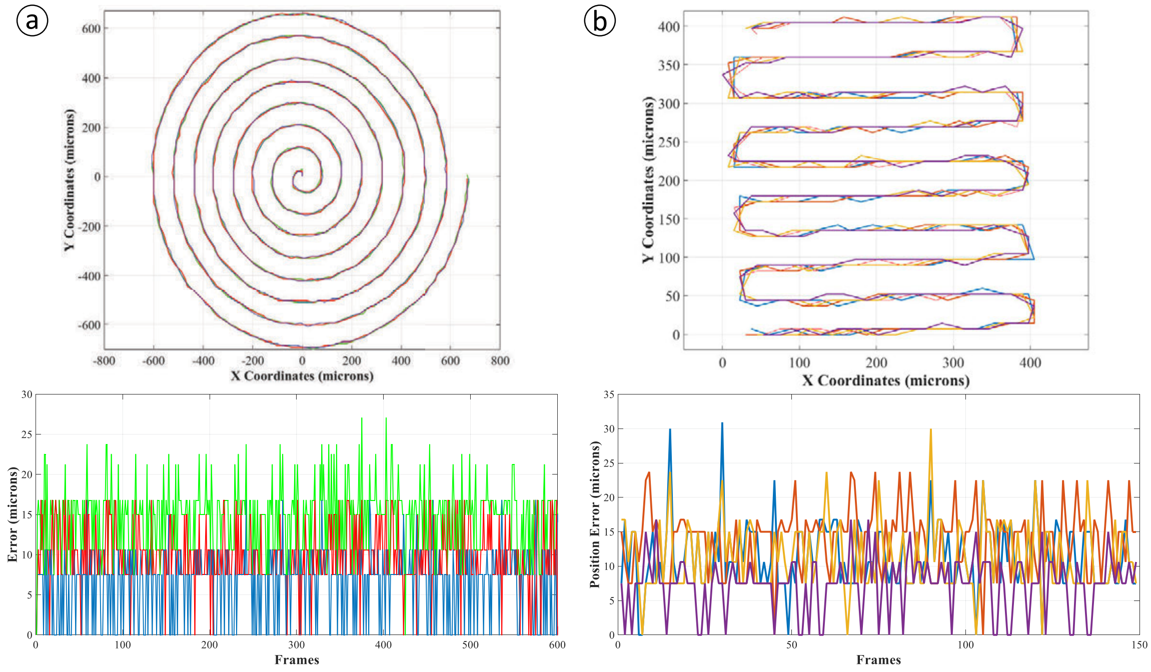


**Figure S6.** Repeatability evaluation of two different scanning patterns along with the corresponding trajectory errors relative to the commanded trajectory, (a) three repeats of spiral trajectories, (b) four repeats of raster trajectories.

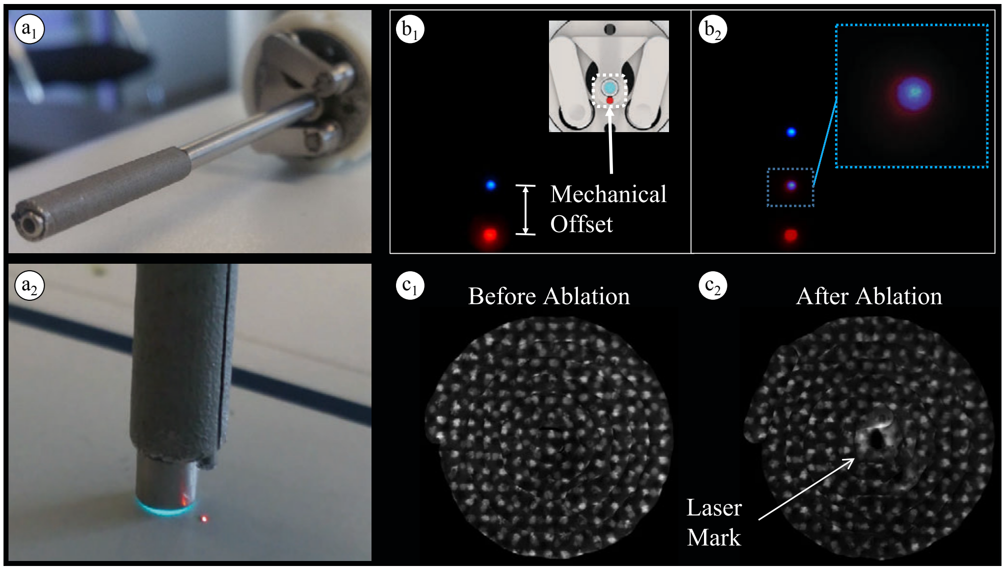


**Figure S7.** ($a_1$) Tip of the instrument showing the $CO_2$ laser and endomicroscopy fibres; ($a_2$) laser firing at a paper card target; ($b_1$) image from the custom tracking rig showing the mechanical offset between the $CO_2$ fibre (red) and the microscopy fibre (blue); ($b_2$) two images, with and without the applied offset correction, overlaid, showing the $CO_2$ laser moves to coincide with the initial position of the endomicroscope; a real-time mosaic, from the same region of the paper card, ($c_1$) before and ($c_2$) after ablation in the centre of the spiral pattern.

## 5 Energy Delivery Offset Calibration

The $CO_2$ laser ablation fibre is inserted through the same channel as the microscopy fibre bundle and is separated by a small horizontal mechanical offset at the tip of the instrument (see Fig. S7(a)). In order to be able to ablate at the centre of the microscopy mosaic, the reverse offset is applied to the probe's position during $CO_2$ laser firing. To determine this offset, the custom tracking rig was used, with $CO_2$ laser replaced with a multi-mode fibre coupled to a red LED to make it visible on the camera. The required offset in voltage space was found (by trial and error) so that the position of the fibre representing the $CO_2$ fibre after the offset was applied coincided with the initial (i.e. non-offset) position of the blue circle corresponding to the endomicrosopy probe position (see Fig. S7(b)). To validate the previous approach, a $CO_2$ laser pulse was fired at the centre of an area that has been mosaicked using a spiral pattern and then it was mosaicked again. Fig. S7(c) shows the area before and after the ablation. The laser mark, as expected, is at the centre of the mosaic.

## References

1. Yuen, HK and Princen, J. and Illingworth, J. and Kittler, J. Comparative study of Hough Transform methods for circle finding *Image and Vision Computing* **8**, 71–77 (1990). DOI 10.1016/0262-8856(90)90059-E.
